# Supplementary material for: MakeAnything: Harnessing Diffusion Transformers for Multi-Domain Procedural Sequence Generation
Source: arXiv:2502.01572 source file (2025-02-05)
Supplement: Supplementary file 1 [file X_suppl.tex]

\clearpage
\setcounter{page}{1}
\maketitlesupplementary

\section{Experimental Details in Different Bench}
\label{sec:rationale}

On each benchmark, the similarity scores are computed between a reference image and two candidate images, one of which is closer to the reference image. Image pair with the higher score is selected as the choice of current evaluated model. In this section, we will explain details of reference and candidate images selection for each benchmark.

\subsection{NIGHTS Dataset}
NIGHTS (Novel Image Generations with Human-Tested Similarities) is a dataset comprising 20,019 image triplets with human scores of perceptual similarity. Each triplet consists of a reference image and two distortions. This paper utilizes the test set of NIGHTS, which includes 2,120 image triplets. We calculate the DiffSim score for the reference image and the two distortions separately, using human evaluation results as the ground truth.

\subsection{Dreambench++ Dataset}

The Dreambench++ Dataset consists of generated images created using different generation methods, along with human-rated scores for how similar each image is to the original. In our experiment, we use the original image as the reference and randomly select two generated images based on it. The one with the higher human rating is considered closer to the reference. The dataset includes a total of 937 triplets.

\subsection{CUTE Dataset}

The CUTE Dataset includes photos of various instances taken under different lighting and positional conditions. In our experiment, for each category, we repeat the process 10 times: randomly selecting two images of the same instance under the same lighting and one image of a different instance under the same lighting. The two images of the same instance are considered more similar. The dataset contains a total of 1,800 triplets for comparison.

\subsection{IP Bench}

IP Bench contains 299 character classes, each with an original image and six variations generated using different consistency weights. In our experiment, we repeat the process for 5 times: using the original image as the reference and randomly selecting two generated images from the same class. The image with the higher consistency weight is considered closer to the reference. There are a total of 1,495 triplets for comparisons.

\subsection{TID2013 Dataset}

The TID2013 dataset contains 25 reference images, each distorted using 24 types of distortions at 5 different levels. In our experiment, we use a reference image as the starting point and randomly select two distorted images using the same type of distortions from the same reference. The image with a lower distortion level is considered closer to the reference. There are a total of 600 triplets for evaluation.

\subsection{Sref Dataset}

The Sref bench includes 508 styles manually selected by artists and generated by Midjounery, with each style featuring four images. When constructing image triplets, we randomly select two images from the same style and one image from a different style. We fix the random seed to construct 2,000 image triplets for quantitative evaluation.

\subsection{InstantStyle Bench}
The InstantStyle bench includes 30 styles, with each style comprising five images. When constructing image triplets, we randomly select two images from the same style and one image from a different style. We fix the random seed to construct 2,000 image triplets for quantitative evaluation.

\subsection{TikTok Dataset}

For tiktok dataset, we extract 10 frames from each video, and calculate the variance of different similarity metric scores between the first frame and other frame. A lower variance indicates that the metric demonstrates better robustness to changes in the movements of characters in the video.

\begin{table*}[ht]
\centering
\caption{Performance of diffsim across various benchmarks with different pre-trained models. Best results are highlighted in bold.}
\label{tab:5}
\small 
\begin{tabular}{@{}c|cc|cc|c|cc@{}}
\toprule
\textbf{Model / Benchmark} & \multicolumn{2}{c|}{\textbf{Human-align Similarity}} & \multicolumn{2}{c|}{\textbf{Instance Similarity}} & \multicolumn{1}{c|}{\textbf{Low-level Similarity}} & \multicolumn{2}{c}{\textbf{Style Similarity}} \\ 
 & \textbf{NIGHTS} & \textbf{Dreambench++} & \textbf{CUTE} & \textbf{IP} & \textbf{TID2013} & \textbf{Sref}  & \textbf{InstantStyle bench} \\ \midrule
DiffSim-S SD1.5                     & \textbf{86.52\%} & \textbf{71.50}\% & 72.06\% & \textbf{92.04\%} & \textbf{94.17\%} & \textbf{97.40\%} & \textbf{99.05\%} \\
DiffSim-C SD1.5                      & 79.16\% & 67.45\% & \textbf{76.17}\% & 77.06\% & 94.00\% & 94.70\% & 95.10\% \\
DiffSim-S SD-XL                      & 78.05\% & 63.93\% & 69.94\% & 83.41\% & 91.33\% & 93.05\% & 96.55\% \\
DiffSim DIT-XL/2 256                 & 63.38\% & 57.52\% & 53.44\% & 82.81\% & 83.50\% & 77.00\% & 80.15\% \\
DiffSim DIT-XL/2 512                 & 67.92\% & 57.31\% & 57.22\% & 81.00\% & 88.67\% & 78.20\% & 79.40\% \\
\bottomrule
\end{tabular}
\end{table*}

\section{Exploring Different Model Architectures}

In Table ~\ref{tab:5}, we present the performance differences of DiffSim using pre-trained models with different architectures. DiffSim-S SD1.5 leads in all benchmarks except for the CUTE dataset. DiffSim-C SD1.5 performs better on the CUTE dataset, possibly because the cross-attention layers in the U-Net architecture are particularly effective at distinguishing the subject. On the other hand, DiffSim-C uses IP-Adapter Plus, and the CLIP image encoder may become a performance bottleneck in other benchmarks. Models with higher resolution, such as SD-XL and DIT-XL/2 512, do not show performance improvement compared to lower resolution models like SD1.5 and DIT-XL/2 256. Furthermore, the performance of models using DIT as the pre-trained model is worse than using U-Net, with two possible reasons: 1. DIT splits the image into patches and then serializes them, which may lead to the loss of spatial information, which is detrimental to DiffSim, despite the use of positional encoding. 2. DIT is trained on the ImageNet dataset, which is much smaller than the SD1.5 and SD-XL models' training datasets.

\section{Additional Experimental Results}
In Figures \ref{nightsbench} to \ref{instantstylebench} , we present the default implementation of DiffSim, which is based on the self-attention layers of SD1.5, showing results across different layers and denoising time steps t.
% 更多实验结果
% 图7-图12，我们展示DiffSim的默认实现，即基于 SD1.5的self attention层中的实现， 不同层和去噪时间步t的结果。
% Additional Experimental Results
% In Figures 7 to 12, we present the default implementation of DiffSim, which is based on the self-attention layers of SD1.5, showing results across different layers and denoising time steps t.

\section{Additional Visual Examples}
Figure ~\ref{supp:bench} and ~\ref{supp:IP} show more examples of images from Sref bench and IP bench; Figure ~\ref{supp:retrieval} presents more top-4 retrieval results of DiffSim, CLIP, DINO v2 on MS COCO, Sref bench and IP bench.

\begin{figure}[htp]
    \centering
    \includegraphics[width=1.0\linewidth]{sec/Image/NIGHTS_Dataset_Performance.pdf}
    \caption{Results on NIGHTS dataset.}
    \label{nightsbench}
\end{figure}

\begin{figure}[htp]
    \centering
    \includegraphics[width=1.0\linewidth]{sec/Image/Dreambench_Dataset_Performance.pdf}
    \caption{Results on Dreambench++ dataset.}
    \label{bench}
\end{figure}

\begin{figure}[htp]
    \centering
    \includegraphics[width=1.0\linewidth]{sec/Image/CUTE_Dataset_Performance.pdf}
    \caption{Results on CUTE dataset.}
    \label{bench}
\end{figure}

\begin{figure}[htp]
    \centering
    \includegraphics[width=1.0\linewidth]{sec/Image/IP_Bench_Performance.pdf}
    \caption{Results on IP bench.}
    \label{bench}
\end{figure}

\begin{figure}[htp]
    \centering
    \includegraphics[width=1.0\linewidth]{sec/Image/TID2013_Performance.pdf}
    \caption{Results on TID2013 dataset.}
    \label{bench}
\end{figure}

\begin{figure}[htp]
    \centering
    \includegraphics[width=1.0\linewidth]{sec/Image/Sref_Bench_Performance.pdf}
    \caption{Results on Sref bench.}
    \label{bench}
\end{figure}

\begin{figure}[htp]
    \centering
    \includegraphics[width=1.0\linewidth]{sec/Image/InstantStyle_Bench_Performance.pdf}
    \caption{Results on InstantStyle bench.}
    \label{instantstylebench}
\end{figure}

\begin{figure*}[htp]
    \centering
    \includegraphics[width=0.89\linewidth]{sec/Image/Sref1.jpg}
    \caption{Examples in Sref bench we proposed.}
    \label{supp:bench}
\end{figure*}

\begin{figure*}[htp]
    \centering
    \includegraphics[width=0.89\linewidth]{sec/Image/IPref.pdf}
    \caption{Examples in IP bench we proposed.}
    \label{supp:IP}
\end{figure*}

\begin{figure*}[htp]
    \centering
    \includegraphics[width=0.99\linewidth]{sec/Image/Supp-ImageRetrieval.pdf}
    \caption{More image retrieval results.}
    \label{supp:retrieval}
\end{figure*}
